# Supplementary material for: CrossNet: Latent Cross-Consistency for Unpaired Image Translation
Source: arXiv:1901.04530 source file (2019-05-26)
Supplement: Supplementary file 1 [file suppmat.tex]

\section{Supplementary Material}

\begin{figure*}[ht]
\begin{tabular}{lccc}

& \hspace{5px} Input \hspace{25px} \OurName & \hspace{5px} Input \hspace{25px} \OurName & \hspace{5px} Input \hspace{25px} \OurName \\

\multirow{2}{*}{\vtop{\hbox{\strut Monet $\rightarrow$}\hbox{\strut Photo}}} &
\raisebox{0\height}{\includegraphics[width=0.125\linewidth]{../Figures/00010_inputA.png}} \raisebox{0\height}{\includegraphics[width=0.125\linewidth]{../Figures/00010_fakeB_IDT3_T3_TIDT6_TCYC6.png}} &
\raisebox{0\height}{\includegraphics[width=0.125\linewidth]{../Figures/00049_inputA.png}} \raisebox{0\height}{\includegraphics[width=0.125\linewidth]{../Figures/00049_fakeB_IDT3_T3_TIDT6_TCYC6.png}} &
\raisebox{0\height}{\includegraphics[width=0.125\linewidth]{../Figures/00047_inputA.png}} \raisebox{0\height}{\includegraphics[width=0.125\linewidth]{../Figures/00047_fakeB_IDT3_T3_TIDT6_TCYC6.png}} \\

&
\raisebox{0\height}{\includegraphics[width=0.125\linewidth]{../Figures/00280_real_A.png}} \raisebox{0\height}{\includegraphics[width=0.125\linewidth]{../Figures/00280_fake_B.png}} &
\raisebox{0\height}{\includegraphics[width=0.125\linewidth]{../Figures/00150_real_A.png}} \raisebox{0\height}{\includegraphics[width=0.125\linewidth]{../Figures/00150_fake_B.png}} &
\raisebox{0\height}{\includegraphics[width=0.125\linewidth]{../Figures/00430_real_A.png}} \raisebox{0\height}{\includegraphics[width=0.125\linewidth]{../Figures/00430_fake_B.png}} \\

\multirow{2}{*}{\vtop{\hbox{\strut Photo $\rightarrow$}\hbox{\strut Monet}}} &
\raisebox{0\height}{\includegraphics[width=0.125\linewidth]{../Figures/00040_inputB.png}} \raisebox{0\height}{\includegraphics[width=0.125\linewidth]{../Figures/00040_fakeA_IDT3_T3_TIDT6_TCYC6.png}} &
\raisebox{0\height}{\includegraphics[width=0.125\linewidth]{../Figures/00050_inputB.png}} \raisebox{0\height}{\includegraphics[width=0.125\linewidth]{../Figures/00050_fakeA_IDT3_T3_TIDT6_TCYC6.png}} &
\raisebox{0\height}{\includegraphics[width=0.125\linewidth]{../Figures/00070_inputB.png}} \raisebox{0\height}{\includegraphics[width=0.125\linewidth]{../Figures/00070_fake_A_IDT3_T3_TIDT6_TCYC6.png}} \\

&
\raisebox{0\height}{\includegraphics[width=0.125\linewidth]{../Figures/00120_real_B.png}} \raisebox{0\height}{\includegraphics[width=0.125\linewidth]{../Figures/00120_fake_A.png}} &
\raisebox{0\height}{\includegraphics[width=0.125\linewidth]{../Figures/00440_real_B.png}} \raisebox{0\height}{\includegraphics[width=0.125\linewidth]{../Figures/00440_fake_A.png}} &
\raisebox{0\height}{\includegraphics[width=0.125\linewidth]{../Figures/00450_real_B.png}} \raisebox{0\height}{\includegraphics[width=0.125\linewidth]{../Figures/00450_fake_A.png}} \\ \\

\multirow{2}{*}{\vtop{\hbox{\strut Cezanne $\rightarrow$}\hbox{\strut Photo}}} &
\raisebox{0\height}{\includegraphics[width=0.125\linewidth]{../Figures/00053_inputA.png}} \raisebox{0\height}{\includegraphics[width=0.125\linewidth]{../Figures/00053_fakeB_IDT3_T3_TIDT6_TCYC6.png}} &
\raisebox{0\height}{\includegraphics[width=0.125\linewidth]{../Figures/00084_inputA.png}} \raisebox{0\height}{\includegraphics[width=0.125\linewidth]{../Figures/00084_fakeB_IDT3_T3_TIDT6_TCYC6.png}} &
\raisebox{0\height}{\includegraphics[width=0.125\linewidth]{../Figures/00006_inputA.png}} \raisebox{0\height}{\includegraphics[width=0.125\linewidth]{../Figures/00006_fakeB_IDT3_T3_TIDT6_TCYC6.png}} \\

&
\raisebox{0\height}{\includegraphics[width=0.125\linewidth]{../Figures/00053_real_A.png}} \raisebox{0\height}{\includegraphics[width=0.125\linewidth]{../Figures/00053_fake_B.png}} &
\raisebox{0\height}{\includegraphics[width=0.125\linewidth]{../Figures/00087_real_A.png}} \raisebox{0\height}{\includegraphics[width=0.125\linewidth]{../Figures/00087_fake_B.png}} &
\raisebox{0\height}{\includegraphics[width=0.125\linewidth]{../Figures/00100_real_A.png}} \raisebox{0\height}{\includegraphics[width=0.125\linewidth]{../Figures/00100_fake_B.png}} \\

\multirow{2}{*}{\vtop{\hbox{\strut Photo $\rightarrow$}\hbox{\strut Cezanne}}} &
\raisebox{0\height}{\includegraphics[width=0.125\linewidth]{../Figures/00070_inputB.png}} \raisebox{0\height}{\includegraphics[width=0.125\linewidth]{../Figures/00070_fake_A_IDT3_T3_TIDT6_TCYC6.png}} &
\raisebox{0\height}{\includegraphics[width=0.125\linewidth]{../Figures/00200_inputB.png}} \raisebox{0\height}{\includegraphics[width=0.125\linewidth]{../Figures/00200_fakeA_IDT3_T3_TIDT6_TCYC6.png}} &
\raisebox{0\height}{\includegraphics[width=0.125\linewidth]{../Figures/00510_inputB.png}} \raisebox{0\height}{\includegraphics[width=0.125\linewidth]{../Figures/00510_fakeA_IDT3_T3_TIDT6_TCYC6.png}} \\

&
\raisebox{0\height}{\includegraphics[width=0.125\linewidth]{../Figures/00510_real_B.png}} \raisebox{0\height}{\includegraphics[width=0.125\linewidth]{../Figures/00510_fake_A.png}} &
\raisebox{0\height}{\includegraphics[width=0.125\linewidth]{../Figures/00520_real_B.png}} \raisebox{0\height}{\includegraphics[width=0.125\linewidth]{../Figures/00520_fake_A.png}} &
\raisebox{0\height}{\includegraphics[width=0.125\linewidth]{../Figures/00530_real_B.png}} \raisebox{0\height}{\includegraphics[width=0.125\linewidth]{../Figures/00530_fake_A.png}} \\

\end{tabular}
\caption{A variety of image-to-image translation results of our method (\OurName), applied on style transfer tasks.}
\label{tab:c2VsCG_Supp}
\end{figure*}

\begin{figure*}[ht]
\begin{tabular}{cccc|cccc}

\multicolumn{4}{c}{Specular to Diffuse} & \multicolumn{4}{c}{Diffuse to Specular} \\

Input & \OurName & Input & \OurName & Input & \OurName & Input & \OurName \\

\includegraphics[width=0.1\linewidth]{../Figures/angel34_512_1035_real_A.png} &
\includegraphics[width=0.1\linewidth]{../Figures/angel34_512_1035_fake_B.png} &
\includegraphics[width=0.1\linewidth]{../Figures/IMG_0408_4_5__512_real_A.png} &
\includegraphics[width=0.1\linewidth]{../Figures/IMG_0408_4_5__512_fake_B.png} &
\includegraphics[width=0.1\linewidth]{../Figures/IMG_0970_4_5__512_real_B.png} &
\includegraphics[width=0.1\linewidth]{../Figures/IMG_0970_4_5__512_fake_A.png} &
\includegraphics[width=0.1\linewidth]{../Figures/IMG_0345_4_5__512_real_B.png} &
\includegraphics[width=0.1\linewidth]{../Figures/IMG_0345_4_5__512_fake_A.png} \\

\includegraphics[width=0.1\linewidth]{../Figures/IMG_0564_4_5__512_real_A.png} &
\includegraphics[width=0.1\linewidth]{../Figures/IMG_0564_4_5__512_fake_B.png} &
\includegraphics[width=0.1\linewidth]{../Figures/jeIMG_0316__512_real_A.png} &
\includegraphics[width=0.1\linewidth]{../Figures/jeIMG_0316__512_fake_B.png} &
\includegraphics[width=0.1\linewidth]{../Figures/IMG_0408_4_5__512_real_B.png} &
\includegraphics[width=0.1\linewidth]{../Figures/IMG_0408_4_5__512_fake_A.png} &
\includegraphics[width=0.1\linewidth]{../Figures/IMG_0220_4_5__512_real_B.png} &
\includegraphics[width=0.1\linewidth]{../Figures/IMG_0220_4_5__512_fake_A.png} \\

\includegraphics[width=0.1\linewidth]{../Figures/IMG_0533_4_5__512_real_A.png} &
\includegraphics[width=0.1\linewidth]{../Figures/IMG_0533_4_5__512_fake_B.png} &
\includegraphics[width=0.1\linewidth]{../Figures/jeIMG_0415__512_real_A.png} &
\includegraphics[width=0.1\linewidth]{../Figures/jeIMG_0415__512_fake_B.png} &
\includegraphics[width=0.1\linewidth]{../Figures/jeIMG_1308__512_real_B.png} &
\includegraphics[width=0.1\linewidth]{../Figures/jeIMG_1308__512_fake_A.png} &
\includegraphics[width=0.1\linewidth]{../Figures/IMG_0377_4_5__512_real_B.png} &
\includegraphics[width=0.1\linewidth]{../Figures/IMG_0377_4_5__512_fake_A.png} \\

\includegraphics[width=0.1\linewidth]{../Figures/angel34_512_1035_real_A.png} &
\includegraphics[width=0.1\linewidth]{../Figures/angel34_512_1035_fake_B.png} &
\includegraphics[width=0.1\linewidth]{../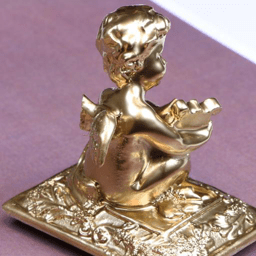} &
\includegraphics[width=0.1\linewidth]{../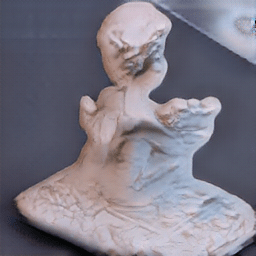} &
\includegraphics[width=0.1\linewidth]{../Figures/IMG_0220_4_5__512_real_B.png} &
\includegraphics[width=0.1\linewidth]{../Figures/IMG_0220_4_5__512_fake_A.png} &
\includegraphics[width=0.1\linewidth]{../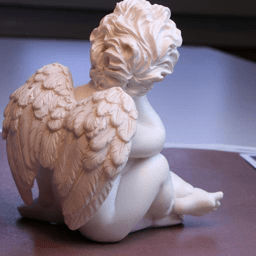} &
\includegraphics[width=0.1\linewidth]{../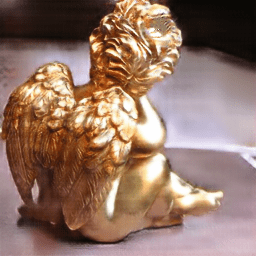} \\

\includegraphics[width=0.1\linewidth]{../Figures/IMG_0002_4_5__512_real_A.png} &
\includegraphics[width=0.1\linewidth]{../Figures/IMG_0002_4_5__512_fake_B.png} &
\includegraphics[width=0.1\linewidth]{../Figures/IMG_0408_4_5__512_real_A.png} &
\includegraphics[width=0.1\linewidth]{../Figures/IMG_0408_4_5__512_fake_B.png} &
\includegraphics[width=0.1\linewidth]{../Figures/IMG_0283_4_5__512_real_B.png} &
\includegraphics[width=0.1\linewidth]{../Figures/IMG_0283_4_5__512_fake_A.png} &
\includegraphics[width=0.1\linewidth]{../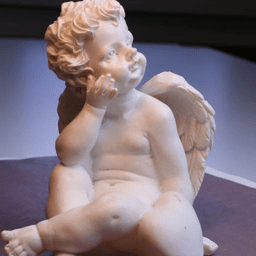} &
\includegraphics[width=0.1\linewidth]{../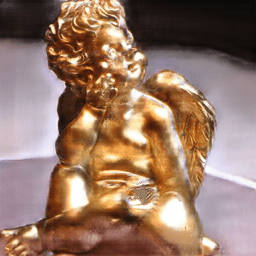} \\

\includegraphics[width=0.1\linewidth]{../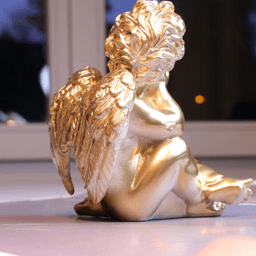} &
\includegraphics[width=0.1\linewidth]{../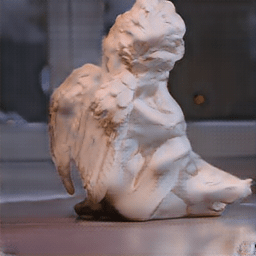} &
\includegraphics[width=0.1\linewidth]{../Figures/IMG_0627_4_5__512_real_A.png} &
\includegraphics[width=0.1\linewidth]{../Figures/IMG_0627_4_5__512_fake_B.png} &
\includegraphics[width=0.1\linewidth]{../Figures/IMG_0345_4_5__512_real_B.png} &
\includegraphics[width=0.1\linewidth]{../Figures/IMG_0345_4_5__512_fake_A.png} &
\includegraphics[width=0.1\linewidth]{../Figures/IMG_0377_4_5__512_real_B.png} &
\includegraphics[width=0.1\linewidth]{../Figures/IMG_0377_4_5__512_fake_A.png} \\

\includegraphics[width=0.1\linewidth]{../Figures/IMG_0533_4_5__512_real_A.png} &
\includegraphics[width=0.1\linewidth]{../Figures/IMG_0533_4_5__512_fake_B.png} &
\includegraphics[width=0.1\linewidth]{../Figures/jeIMG_0415__512_real_A.png} &
\includegraphics[width=0.1\linewidth]{../Figures/jeIMG_0415__512_fake_B.png} &
\includegraphics[width=0.1\linewidth]{../Figures/IMG_0408_4_5__512_real_B.png} &
\includegraphics[width=0.1\linewidth]{../Figures/IMG_0408_4_5__512_fake_A.png} &
\includegraphics[width=0.1\linewidth]{../Figures/jeIMG_0003__512_real_B.png} &
\includegraphics[width=0.1\linewidth]{../Figures/jeIMG_0003__512_fake_A.png} \\

\includegraphics[width=0.1\linewidth]{../Figures/IMG_0564_4_5__512_real_A.png} &
\includegraphics[width=0.1\linewidth]{../Figures/IMG_0564_4_5__512_fake_B.png} &
\includegraphics[width=0.1\linewidth]{../Figures/jeIMG_0316__512_real_A.png} &
\includegraphics[width=0.1\linewidth]{../Figures/jeIMG_0316__512_fake_B.png} &
\includegraphics[width=0.1\linewidth]{../Figures/IMG_0970_4_5__512_real_B.png} &
\includegraphics[width=0.1\linewidth]{../Figures/IMG_0970_4_5__512_fake_A.png} &
\includegraphics[width=0.1\linewidth]{../Figures/jeIMG_1308__512_real_B.png} &
\includegraphics[width=0.1\linewidth]{../Figures/jeIMG_1308__512_fake_A.png} \\

\end{tabular}
\caption{Results of our Specular to Diffuse: The odd colums show the inputs while the even ones show our output. The four left most columns depict a translation form a specular input to a diffuse output, while the four right rows show the opposite direction of translation.}
\end{figure*}

\begin{figure*}[ht]
\begin{tabular}{ccccc}

Input & \OurName & CycleGAN & MUNIT & DPED \\

\includegraphics[width=0.175\linewidth]{../Figures/107_real_A_Overlay.png} &
\includegraphics[width=0.175\linewidth]{../Figures/107_fake_B_Ours_Overlay.png} &
\includegraphics[width=0.175\linewidth]{../Figures/107_fake_B_CG_Overlay.png} &
\includegraphics[width=0.175\linewidth]{../Figures/107_fake_B_MUNIT_Overlay.png} & 
\includegraphics[width=0.175\linewidth]{../Figures/107_fake_B_DPED_Overlay.png} \\

\includegraphics[width=0.175\linewidth]{../Figures/107_real_A_Zoom.png} &
\includegraphics[width=0.175\linewidth]{../Figures/107_fake_B_Ours_Zoom.png} &
\includegraphics[width=0.175\linewidth]{../Figures/107_fake_B_CG_Zoom.png} &
\includegraphics[width=0.175\linewidth]{../Figures/107_fake_B_MUNIT_Zoom.png} &
\includegraphics[width=0.175\linewidth]{../Figures/107_fake_B_DPED_Zoom.png} \\

\includegraphics[width=0.175\linewidth]{../Figures/1002_real_A_Overlay.png} &
\includegraphics[width=0.175\linewidth]{../Figures/1002_fake_B_Ours_Overlay.png} &
\includegraphics[width=0.175\linewidth]{../Figures/1002_fake_B_CG_Overlay.png} &
\includegraphics[width=0.175\linewidth]{../Figures/1002_fake_B_MUNIT_Overlay.png} & 
\includegraphics[width=0.175\linewidth]{../Figures/1002_fake_B_DPED_Overlay.png} \\

\includegraphics[width=0.175\linewidth]{../Figures/1002_real_A_Zoom.png} &
\includegraphics[width=0.175\linewidth]{../Figures/1002_fake_B_Ours_Zoom.png} &
\includegraphics[width=0.175\linewidth]{../Figures/1002_fake_B_CG_Zoom.png} &
\includegraphics[width=0.175\linewidth]{../Figures/1002_fake_B_MUNIT_Zoom.png} &
\includegraphics[width=0.175\linewidth]{../Figures/1002_fake_B_DPED_Zoom.png} \\

\includegraphics[width=0.175\linewidth]{../Figures/1042_real_A_Overlay.png} &
\includegraphics[width=0.175\linewidth]{../Figures/1042_fake_B_Ours_Overlay.png} &
\includegraphics[width=0.175\linewidth]{../Figures/1042_fake_B_CG_Overlay.png} &
\includegraphics[width=0.175\linewidth]{../Figures/1042_fake_B_MUNIT_Overlay.png} & 
\includegraphics[width=0.175\linewidth]{../Figures/1042_fake_B_DPED_Overlay.png} \\

\includegraphics[width=0.175\linewidth]{../Figures/1042_real_A_Zoom.png} &
\includegraphics[width=0.175\linewidth]{../Figures/1042_fake_B_Ours_Zoom.png} &
\includegraphics[width=0.175\linewidth]{../Figures/1042_fake_B_CG_Zoom.png} &
\includegraphics[width=0.175\linewidth]{../Figures/1042_fake_B_MUNIT_Zoom.png} &
\includegraphics[width=0.175\linewidth]{../Figures/1042_fake_B_DPED_Zoom.png} \\

\end{tabular}
\caption{Results of employing \OurName for enhancing a mobile phone photo to DSLR quality. We show the input, our result, Cycle GAN's, MUNIT's and DPED's results, from left to right. The odd rows show the full images, while the even rows show a zoom-in.}
\end{figure*}

\begin{figure*}[ht]
\begin{tabular}{ccccc}

Input & \OurName & CycleGAN & MUNIT & DPED \\

\includegraphics[width=0.175\linewidth]{../Figures/1046_real_A_Overlay.png} &
\includegraphics[width=0.175\linewidth]{../Figures/1046_fake_B_Ours_Overlay.png} &
\includegraphics[width=0.175\linewidth]{../Figures/1046_fake_B_CG_Overlay.png} &
\includegraphics[width=0.175\linewidth]{../Figures/1046_fake_B_MUNIT_Overlay.png} & 
\includegraphics[width=0.175\linewidth]{../Figures/1046_fake_B_DPED_Overlay.png} \\

\includegraphics[width=0.175\linewidth]{../Figures/1046_real_A_Zoom.png} &
\includegraphics[width=0.175\linewidth]{../Figures/1046_fake_B_Ours_Zoom.png} &
\includegraphics[width=0.175\linewidth]{../Figures/1046_fake_B_CG_Zoom.png} &
\includegraphics[width=0.175\linewidth]{../Figures/1046_fake_B_MUNIT_Zoom.png} &
\includegraphics[width=0.175\linewidth]{../Figures/1046_fake_B_DPED_Zoom.png} \\

\includegraphics[width=0.175\linewidth]{../Figures/1068_real_A_Overlay.png} &
\includegraphics[width=0.175\linewidth]{../Figures/1068_fake_B_Ours_Overlay.png} &
\includegraphics[width=0.175\linewidth]{../Figures/1068_fake_B_CG_Overlay.png} &
\includegraphics[width=0.175\linewidth]{../Figures/1068_fake_B_MUNIT_Overlay.png} & 
\includegraphics[width=0.175\linewidth]{../Figures/1068_fake_B_DPED_Overlay.png} \\

\includegraphics[width=0.175\linewidth]{../Figures/1068_real_A_Zoom.png} &
\includegraphics[width=0.175\linewidth]{../Figures/1068_fake_B_Ours_Zoom.png} &
\includegraphics[width=0.175\linewidth]{../Figures/1068_fake_B_CG_Zoom.png} &
\includegraphics[width=0.175\linewidth]{../Figures/1068_fake_B_MUNIT_Zoom.png} &
\includegraphics[width=0.175\linewidth]{../Figures/1068_fake_B_DPED_Zoom.png} \\

\includegraphics[width=0.175\linewidth]{../Figures/1071_real_A_Overlay.png} &
\includegraphics[width=0.175\linewidth]{../Figures/1071_fake_B_Ours_Overlay.png} &
\includegraphics[width=0.175\linewidth]{../Figures/1071_fake_B_CG_Overlay.png} &
\includegraphics[width=0.175\linewidth]{../Figures/1071_fake_B_MUNIT_Overlay.png} & 
\includegraphics[width=0.175\linewidth]{../Figures/1071_fake_B_DPED_Overlay.png} \\

\includegraphics[width=0.175\linewidth]{../Figures/1071_real_A_Zoom.png} &
\includegraphics[width=0.175\linewidth]{../Figures/1071_fake_B_Ours_Zoom.png} &
\includegraphics[width=0.175\linewidth]{../Figures/1071_fake_B_CG_Zoom.png} &
\includegraphics[width=0.175\linewidth]{../Figures/1071_fake_B_MUNIT_Zoom.png} &
\includegraphics[width=0.175\linewidth]{../Figures/1071_fake_B_DPED_Zoom.png} \\

\end{tabular}
\caption{Results of employing \OurName for enhancing a mobile phone photo to DSLR quality. We show the input, our result, Cycle GAN's, MUNIT's and DPED's results, from left to right. The odd rows show the full images, while the even rows show a zoom-in.}
\end{figure*}

\begin{figure*}[ht]
\begin{tabular}{cccc|cccc}

Input & \OurName & CycleGAN & GrabCut & Input & \OurName & CycleGAN & GrabCut \\

\includegraphics[width=0.1\linewidth]{../Figures/ElephantWOBG_0004_real_B.png} &
\includegraphics[width=0.1\linewidth]{../Figures/ElephantWOBG_0004_fake_A_procd.png} &
\includegraphics[width=0.1\linewidth]{../Figures/ElephantWOBG_0004_fake_A_procd_CG.png} &
\includegraphics[width=0.1\linewidth]{../Figures/ElephantWOBG_0004_fake_A_Grabcut.png} &
\includegraphics[width=0.1\linewidth]{../Figures/ElephantWOBG_0018_real_B.png} &
\includegraphics[width=0.1\linewidth]{../Figures/ElephantWOBG_0018_fake_A_procd.png} &
\includegraphics[width=0.1\linewidth]{../Figures/ElephantWOBG_0018_fake_A_procd_CG.png} &
\includegraphics[width=0.1\linewidth]{../Figures/ElephantWOBG_0018_fake_A_Grabcut.png} \\

\includegraphics[width=0.1\linewidth]{../Figures/ElephantWOBG_0054_real_B.png} &
\includegraphics[width=0.1\linewidth]{../Figures/ElephantWOBG_0054_fake_A_procd.png} &
\includegraphics[width=0.1\linewidth]{../Figures/ElephantWOBG_0054_fake_A_procd_CG.png} &
\includegraphics[width=0.1\linewidth]{../Figures/ElephantWOBG_0054_fake_A_Grabcut.png} &
\includegraphics[width=0.1\linewidth]{../Figures/ElephantWOBG_0056_real_B.png} &
\includegraphics[width=0.1\linewidth]{../Figures/ElephantWOBG_0056_fake_A_procd.png} &
\includegraphics[width=0.1\linewidth]{../Figures/ElephantWOBG_0056_fake_A_procd_CG.png} &
\includegraphics[width=0.1\linewidth]{../Figures/ElephantWOBG_0056_fake_A_Grabcut.png} \\

\includegraphics[width=0.1\linewidth]{../Figures/ElephantWOBG_0062_real_B.png} &
\includegraphics[width=0.1\linewidth]{../Figures/ElephantWOBG_0062_fake_A_procd.png} &
\includegraphics[width=0.1\linewidth]{../Figures/ElephantWOBG_0062_fake_A_procd_CG.png} &
\includegraphics[width=0.1\linewidth]{../Figures/ElephantWOBG_0062_fake_A_Grabcut.png} &
\includegraphics[width=0.1\linewidth]{../Figures/ElephantWOBG_0063_real_B.png} &
\includegraphics[width=0.1\linewidth]{../Figures/ElephantWOBG_0063_fake_A_procd.png} &
\includegraphics[width=0.1\linewidth]{../Figures/ElephantWOBG_0063_fake_A_procd_CG.png} &
\includegraphics[width=0.1\linewidth]{../Figures/ElephantWOBG_0063_fake_A_Grabcut.png} \\

\includegraphics[width=0.1\linewidth]{../Figures/ElephantWOBG_0067_real_B.png} &
\includegraphics[width=0.1\linewidth]{../Figures/ElephantWOBG_0067_fake_A_procd.png} &
\includegraphics[width=0.1\linewidth]{../Figures/ElephantWOBG_0067_fake_A_procd_CG.png} &
\includegraphics[width=0.1\linewidth]{../Figures/ElephantWOBG_0067_fake_A_Grabcut.png} &
\includegraphics[width=0.1\linewidth]{../Figures/ElephantWOBG_0083_real_B.png} &
\includegraphics[width=0.1\linewidth]{../Figures/ElephantWOBG_0083_fake_A_procd.png} &
\includegraphics[width=0.1\linewidth]{../Figures/ElephantWOBG_0083_fake_A_procd_CG.png} &
\includegraphics[width=0.1\linewidth]{../Figures/ElephantWOBG_0083_fake_A_Grabcut.png} \\

\includegraphics[width=0.1\linewidth]{../Figures/ElephantWOBG_0121_real_B.png} &
\includegraphics[width=0.1\linewidth]{../Figures/ElephantWOBG_0121_fake_A_procd.png} &
\includegraphics[width=0.1\linewidth]{../Figures/ElephantWOBG_0121_fake_A_procd_CG.png} &
\includegraphics[width=0.1\linewidth]{../Figures/ElephantWOBG_0121_fake_A_Grabcut.png} &
\includegraphics[width=0.1\linewidth]{../Figures/ElephantWOBG_0138_real_B.png} &
\includegraphics[width=0.1\linewidth]{../Figures/ElephantWOBG_0138_fake_A_procd.png} &
\includegraphics[width=0.1\linewidth]{../Figures/ElephantWOBG_0138_fake_A_procd_CG.png} &
\includegraphics[width=0.1\linewidth]{../Figures/ElephantWOBG_0138_fake_A_Grabcut.png} \\

\includegraphics[width=0.1\linewidth]{../Figures/ElephantWOBG_0211_real_B.png} &
\includegraphics[width=0.1\linewidth]{../Figures/ElephantWOBG_0211_fake_A_procd.png} &
\includegraphics[width=0.1\linewidth]{../Figures/ElephantWOBG_0211_fake_A_procd_CG.png} &
\includegraphics[width=0.1\linewidth]{../Figures/ElephantWOBG_0211_fake_A_Grabcut.png} &
\includegraphics[width=0.1\linewidth]{../Figures/ElephantWOBG_0150_real_B.png} &
\includegraphics[width=0.1\linewidth]{../Figures/ElephantWOBG_0150_fake_A_procd.png} &
\includegraphics[width=0.1\linewidth]{../Figures/ElephantWOBG_0150_fake_A_procd_CG.png} &
\includegraphics[width=0.1\linewidth]{../Figures/ElephantWOBG_0150_fake_A_Grabcut.png} \\

\includegraphics[width=0.1\linewidth]{../Figures/ElephantWOBG_0153_real_B.png} &
\includegraphics[width=0.1\linewidth]{../Figures/ElephantWOBG_0153_fake_A_procd.png} &
\includegraphics[width=0.1\linewidth]{../Figures/ElephantWOBG_0153_fake_A_procd_CG.png} &
\includegraphics[width=0.1\linewidth]{../Figures/ElephantWOBG_0153_fake_A_Grabcut.png} &
\includegraphics[width=0.1\linewidth]{../Figures/ElephantWOBG_0155_real_B.png} &
\includegraphics[width=0.1\linewidth]{../Figures/ElephantWOBG_0155_fake_A_procd.png} &
\includegraphics[width=0.1\linewidth]{../Figures/ElephantWOBG_0155_fake_A_procd_CG.png} &
\includegraphics[width=0.1\linewidth]{../Figures/ElephantWOBG_0155_fake_A_Grabcut.png} \\

\includegraphics[width=0.1\linewidth]{../Figures/ElephantWOBG_0157_real_B.png} &
\includegraphics[width=0.1\linewidth]{../Figures/ElephantWOBG_0157_fake_A_procd.png} &
\includegraphics[width=0.1\linewidth]{../Figures/ElephantWOBG_0157_fake_A_procd_CG.png} &
\includegraphics[width=0.1\linewidth]{../Figures/ElephantWOBG_0157_fake_A_Grabcut.png} &
\includegraphics[width=0.1\linewidth]{../Figures/ElephantWOBG_0160_real_B.png} &
\includegraphics[width=0.1\linewidth]{../Figures/ElephantWOBG_0160_fake_A_procd.png} &
\includegraphics[width=0.1\linewidth]{../Figures/ElephantWOBG_0160_fake_A_procd_CG.png} &
\includegraphics[width=0.1\linewidth]{../Figures/ElephantWOBG_0160_fake_A_Grabcut.png} \\

\includegraphics[width=0.1\linewidth]{../Figures/ElephantWOBG_0161_real_B.png} &
\includegraphics[width=0.1\linewidth]{../Figures/ElephantWOBG_0161_fake_A_procd.png} &
\includegraphics[width=0.1\linewidth]{../Figures/ElephantWOBG_0161_fake_A_procd_CG.png} &
\includegraphics[width=0.1\linewidth]{../Figures/ElephantWOBG_0161_fake_A_Grabcut.png} &
\includegraphics[width=0.1\linewidth]{../Figures/ElephantWOBG_0168_real_B.png} &
\includegraphics[width=0.1\linewidth]{../Figures/ElephantWOBG_0168_fake_A_procd.png} &
\includegraphics[width=0.1\linewidth]{../Figures/ElephantWOBG_0168_fake_A_procd_CG.png} &
\includegraphics[width=0.1\linewidth]{../Figures/ElephantWOBG_0168_fake_A_Grabcut.png} \\

\includegraphics[width=0.1\linewidth]{../Figures/ElephantWOBG_0189_real_B.png} &
\includegraphics[width=0.1\linewidth]{../Figures/ElephantWOBG_0189_fake_A_procd.png} &
\includegraphics[width=0.1\linewidth]{../Figures/ElephantWOBG_0189_fake_A_procd_CG.png} &
\includegraphics[width=0.1\linewidth]{../Figures/ElephantWOBG_0189_fake_A_Grabcut.png} &
\includegraphics[width=0.1\linewidth]{../Figures/ElephantWOBG_0181_real_B.png} &
\includegraphics[width=0.1\linewidth]{../Figures/ElephantWOBG_0181_fake_A_procd.png} &
\includegraphics[width=0.1\linewidth]{../Figures/ElephantWOBG_0181_fake_A_procd_CG.png} &
\includegraphics[width=0.1\linewidth]{../Figures/ElephantWOBG_0181_fake_A_Grabcut.png} \\

\includegraphics[width=0.1\linewidth]{../Figures/ElephantWOBG_0198_real_B.png} &
\includegraphics[width=0.1\linewidth]{../Figures/ElephantWOBG_0198_fake_A_procd.png} &
\includegraphics[width=0.1\linewidth]{../Figures/ElephantWOBG_0198_fake_A_procd_CG.png} &
\includegraphics[width=0.1\linewidth]{../Figures/ElephantWOBG_0198_fake_A_Grabcut.png} &
\includegraphics[width=0.1\linewidth]{../Figures/ElephantWOBG_0208_real_B.png} &
\includegraphics[width=0.1\linewidth]{../Figures/ElephantWOBG_0208_fake_A_procd.png} &
\includegraphics[width=0.1\linewidth]{../Figures/ElephantWOBG_0208_fake_A_procd_CG.png} &
\includegraphics[width=0.1\linewidth]{../Figures/ElephantWOBG_0208_fake_A_Grabcut.png} \\

\includegraphics[width=0.1\linewidth]{../Figures/ElephantWOBG_0218_real_B.png} &
\includegraphics[width=0.1\linewidth]{../Figures/ElephantWOBG_0218_fake_A_procd.png} &
\includegraphics[width=0.1\linewidth]{../Figures/ElephantWOBG_0218_fake_A_procd_CG.png} &
\includegraphics[width=0.1\linewidth]{../Figures/ElephantWOBG_0218_fake_A_Grabcut.png} &
\includegraphics[width=0.1\linewidth]{../Figures/ElephantWOBG_0230_real_B.png} &
\includegraphics[width=0.1\linewidth]{../Figures/ElephantWOBG_0230_fake_A_procd.png} &
\includegraphics[width=0.1\linewidth]{../Figures/ElephantWOBG_0230_fake_A_procd_CG.png} &
\includegraphics[width=0.1\linewidth]{../Figures/ElephantWOBG_0230_fake_A_Grabcut.png} \\

\end{tabular}
\caption{Results of employing \OurName for foreground extraction applied on elephant photos. From left to right, we show the input image, CrossNet, CycleGAN and GrabCut.}
\end{figure*}

\begin{figure*}[ht]
\begin{tabular}{cccc|cccc}

Input & \OurName & CycleGAN & AGGAN & Input & \OurName & CycleGAN & AGGAN \\

\includegraphics[width=0.1\linewidth]{../Figures/102121_287_real_B.png} &
\includegraphics[width=0.1\linewidth]{../Figures/102121_287_fake_A_procd_Ours.png} &
\includegraphics[width=0.1\linewidth]{../Figures/102121_287_fake_A_procd_CG.png} &
\includegraphics[width=0.1\linewidth]{../Figures/102121_287_fake_A_procd_AGGAN.png} &

\includegraphics[width=0.1\linewidth]{../Figures/104676_189953_real_B.png} &
\includegraphics[width=0.1\linewidth]{../Figures/104676_189953_fake_A_procd_Ours.png} &
\includegraphics[width=0.1\linewidth]{../Figures/104676_189953_fake_A_procd_CG.png} &
\includegraphics[width=0.1\linewidth]{../Figures/104676_189953_fake_A_procd_AGGAN.png} \\

\includegraphics[width=0.1\linewidth]{../Figures/104676_617_real_B.png} &
\includegraphics[width=0.1\linewidth]{../Figures/104676_617_fake_A_procd_Ours.png} &
\includegraphics[width=0.1\linewidth]{../Figures/104676_617_fake_A_procd_CG.png} &
\includegraphics[width=0.1\linewidth]{../Figures/104676_617_fake_A_procd_AGGAN.png} &

\includegraphics[width=0.1\linewidth]{../Figures/104676_9_real_B.png} &
\includegraphics[width=0.1\linewidth]{../Figures/104676_9_fake_A_procd_Ours.png} &
\includegraphics[width=0.1\linewidth]{../Figures/104676_9_fake_A_procd_CG.png} &
\includegraphics[width=0.1\linewidth]{../Figures/104676_9_fake_A_procd_AGGAN.png} \\

\includegraphics[width=0.1\linewidth]{../Figures/7538282_225096_real_B.png} &
\includegraphics[width=0.1\linewidth]{../Figures/7538282_225096_fake_A_procd_Ours.png} &
\includegraphics[width=0.1\linewidth]{../Figures/7538282_225096_fake_A_procd_CG.png} &
\includegraphics[width=0.1\linewidth]{../Figures/7538282_225096_fake_A_procd_AGGAN.png} &

\includegraphics[width=0.1\linewidth]{../Figures/7212450_20_real_B.png} &
\includegraphics[width=0.1\linewidth]{../Figures/7212450_20_fake_A_procd_Ours.png} &
\includegraphics[width=0.1\linewidth]{../Figures/7212450_20_fake_A_procd_CG.png} &
\includegraphics[width=0.1\linewidth]{../Figures/7212450_20_fake_A_procd_AGGAN.png} \\

\includegraphics[width=0.1\linewidth]{../Figures/7212450_364920_real_B.png} &
\includegraphics[width=0.1\linewidth]{../Figures/7212450_364920_fake_A_procd_Ours.png} &
\includegraphics[width=0.1\linewidth]{../Figures/7212450_364920_fake_A_procd_CG.png} &
\includegraphics[width=0.1\linewidth]{../Figures/7212450_364920_fake_A_procd_AGGAN.png} &

\includegraphics[width=0.1\linewidth]{../Figures/7212459_691_real_B.png} &
\includegraphics[width=0.1\linewidth]{../Figures/7212459_691_fake_A_procd_Ours.png} &
\includegraphics[width=0.1\linewidth]{../Figures/7212459_691_fake_A_procd_CG.png} &
\includegraphics[width=0.1\linewidth]{../Figures/7212459_691_fake_A_procd_AGGAN.png} \\

\includegraphics[width=0.1\linewidth]{../Figures/7271610_11_real_B.png} &
\includegraphics[width=0.1\linewidth]{../Figures/7271610_11_fake_A_procd_Ours.png} &
\includegraphics[width=0.1\linewidth]{../Figures/7271610_11_fake_A_procd_CG.png} &
\includegraphics[width=0.1\linewidth]{../Figures/7271610_11_fake_A_procd_AGGAN.png} &

\includegraphics[width=0.1\linewidth]{../Figures/7373491_4697_real_B.png} &
\includegraphics[width=0.1\linewidth]{../Figures/7373491_4697_fake_A_procd_Ours.png} &
\includegraphics[width=0.1\linewidth]{../Figures/7373491_4697_fake_A_procd_CG.png} &
\includegraphics[width=0.1\linewidth]{../Figures/7373491_4697_fake_A_procd_AGGAN.png} \\

\includegraphics[width=0.1\linewidth]{../Figures/7161124_20_real_B.png} &
\includegraphics[width=0.1\linewidth]{../Figures/7161124_20_fake_A_procd_Ours.png} &
\includegraphics[width=0.1\linewidth]{../Figures/7161124_20_fake_A_procd_CG.png} &
\includegraphics[width=0.1\linewidth]{../Figures/7161124_20_fake_A_procd_AGGAN.png} &

\includegraphics[width=0.1\linewidth]{../Figures/7212450_303655_real_B.png} &
\includegraphics[width=0.1\linewidth]{../Figures/7212450_303655_fake_A_procd_Ours.png} &
\includegraphics[width=0.1\linewidth]{../Figures/7212450_303655_fake_A_procd_CG.png} &
\includegraphics[width=0.1\linewidth]{../Figures/7212450_303655_fake_A_procd_AGGAN.png} \\

\includegraphics[width=0.1\linewidth]{../Figures/7571295_10623_real_B.png} &
\includegraphics[width=0.1\linewidth]{../Figures/7571295_10623_fake_A_procd_Ours.png} &
\includegraphics[width=0.1\linewidth]{../Figures/7571295_10623_fake_A_procd_CG.png} &
\includegraphics[width=0.1\linewidth]{../Figures/7571295_10623_fake_A_procd_AGGAN.png} &

\includegraphics[width=0.1\linewidth]{../Figures/7212450_366115_real_B.png} &
\includegraphics[width=0.1\linewidth]{../Figures/7212450_366115_fake_A_procd_Ours.png} &
\includegraphics[width=0.1\linewidth]{../Figures/7212450_366115_fake_A_procd_CG.png} &
\includegraphics[width=0.1\linewidth]{../Figures/7212450_366115_fake_A_procd_AGGAN.png} \\

\includegraphics[width=0.1\linewidth]{../Figures/7567515_9_real_B.png} &
\includegraphics[width=0.1\linewidth]{../Figures/7567515_9_fake_A_procd_Ours.png} &
\includegraphics[width=0.1\linewidth]{../Figures/7567515_9_fake_A_procd_CG.png} &
\includegraphics[width=0.1\linewidth]{../Figures/7567515_9_fake_A_procd_AGGAN.png} &

\includegraphics[width=0.1\linewidth]{../Figures/7425142_3575_real_B.png} &
\includegraphics[width=0.1\linewidth]{../Figures/7425142_3575_fake_A_procd_Ours.png} &
\includegraphics[width=0.1\linewidth]{../Figures/7425142_3575_fake_A_procd_CG.png} &
\includegraphics[width=0.1\linewidth]{../Figures/7425142_3575_fake_A_procd_AGGAN.png} \\

\includegraphics[width=0.1\linewidth]{../Figures/7158233_3_real_B.png} &
\includegraphics[width=0.1\linewidth]{../Figures/7158233_3_fake_A_procd_Ours.png} &
\includegraphics[width=0.1\linewidth]{../Figures/7158233_3_fake_A_procd_CG.png} &
\includegraphics[width=0.1\linewidth]{../Figures/7158233_3_fake_A_procd_AGGAN.png} &

\includegraphics[width=0.1\linewidth]{../Figures/7159690_89459_real_B.png} &
\includegraphics[width=0.1\linewidth]{../Figures/7159690_89459_fake_A_procd_Ours.png} &
\includegraphics[width=0.1\linewidth]{../Figures/7159690_89459_fake_A_procd_CG.png} &
\includegraphics[width=0.1\linewidth]{../Figures/7159690_89459_fake_A_procd_AGGAN.png} \\

\includegraphics[width=0.1\linewidth]{../Figures/7297622_352714_real_B.png} &
\includegraphics[width=0.1\linewidth]{../Figures/7297622_352714_fake_A_procd_Ours.png} &
\includegraphics[width=0.1\linewidth]{../Figures/7297622_352714_fake_A_procd_CG.png} &
\includegraphics[width=0.1\linewidth]{../Figures/7297622_352714_fake_A_procd_AGGAN.png} &

\includegraphics[width=0.1\linewidth]{../Figures/7289535_4697_real_B.png} &
\includegraphics[width=0.1\linewidth]{../Figures/7289535_4697_fake_A_procd_Ours.png} &
\includegraphics[width=0.1\linewidth]{../Figures/7289535_4697_fake_A_procd_CG.png} &
\includegraphics[width=0.1\linewidth]{../Figures/7289535_4697_fake_A_procd_AGGAN.png} \\

\end{tabular}
\caption{Results of employing \OurName for foreground extraction applied on the UT Zappos50K dataset. From left to right, we show the input image, CrossNet, CycleGAN and AGGAN.}
\end{figure*}

\begin{figure*}[ht]
\begin{tabular}{ccc|ccc}

Input & Ground Truth & \OurName & Input & Ground Truth & \OurName \\

\includegraphics[width=0.13\linewidth]{../Figures/2007_003022_real_B.png} &
\includegraphics[width=0.13\linewidth]{../Figures/2007_003022_real_A.png} &
\includegraphics[width=0.13\linewidth]{../Figures/2007_003022_fake_A_procd.png} &

\includegraphics[width=0.13\linewidth]{../Figures/2007_005114_real_B.png} &
\includegraphics[width=0.13\linewidth]{../Figures/2007_005114_real_A.png} &
\includegraphics[width=0.13\linewidth]{../Figures/2007_005114_fake_A_procd.png} \\

\includegraphics[width=0.13\linewidth]{../Figures/2007_006364_real_B.png} &
\includegraphics[width=0.13\linewidth]{../Figures/2007_006364_real_A.png} &
\includegraphics[width=0.13\linewidth]{../Figures/2007_006364_fake_A_procd.png} &

\includegraphics[width=0.13\linewidth]{../Figures/2008_002459_real_B.png} &
\includegraphics[width=0.13\linewidth]{../Figures/2008_002459_real_A.png} &
\includegraphics[width=0.13\linewidth]{../Figures/2008_002459_fake_A_procd.png} \\

\includegraphics[width=0.13\linewidth]{../Figures/2007_008142_real_B.png} &
\includegraphics[width=0.13\linewidth]{../Figures/2007_008142_real_A.png} &
\includegraphics[width=0.13\linewidth]{../Figures/2007_008142_fake_A_procd.png} &

\includegraphics[width=0.13\linewidth]{../Figures/2007_008256_real_B.png} &
\includegraphics[width=0.13\linewidth]{../Figures/2007_008256_real_A.png} &
\includegraphics[width=0.13\linewidth]{../Figures/2007_008256_fake_A_procd.png} \\

\includegraphics[width=0.13\linewidth]{../Figures/2007_008307_real_B.png} &
\includegraphics[width=0.13\linewidth]{../Figures/2007_008307_real_A.png} &
\includegraphics[width=0.13\linewidth]{../Figures/2007_008307_fake_A_procd.png} &

\includegraphics[width=0.13\linewidth]{../Figures/2007_008802_real_B.png} &
\includegraphics[width=0.13\linewidth]{../Figures/2007_008802_real_A.png} &
\includegraphics[width=0.13\linewidth]{../Figures/2007_008802_fake_A_procd.png} \\

\includegraphics[width=0.13\linewidth]{../Figures/2007_009251_real_B.png} &
\includegraphics[width=0.13\linewidth]{../Figures/2007_009251_real_A.png} &
\includegraphics[width=0.13\linewidth]{../Figures/2007_009251_fake_A_procd.png} &

\includegraphics[width=0.13\linewidth]{../Figures/2007_009807_real_B.png} &
\includegraphics[width=0.13\linewidth]{../Figures/2007_009807_real_A.png} &
\includegraphics[width=0.13\linewidth]{../Figures/2007_009807_fake_A_procd.png} \\

\includegraphics[width=0.13\linewidth]{../Figures/2008_000141_real_B.png} &
\includegraphics[width=0.13\linewidth]{../Figures/2008_000141_real_A.png} &
\includegraphics[width=0.13\linewidth]{../Figures/2008_000141_fake_A_procd.png} &

\includegraphics[width=0.13\linewidth]{../Figures/2008_000219_real_B.png} &
\includegraphics[width=0.13\linewidth]{../Figures/2008_000219_real_A.png} &
\includegraphics[width=0.13\linewidth]{../Figures/2008_000219_fake_A_procd.png} \\

\includegraphics[width=0.13\linewidth]{../Figures/2008_005928_real_B.png} &
\includegraphics[width=0.13\linewidth]{../Figures/2008_005928_real_A.png} &
\includegraphics[width=0.13\linewidth]{../Figures/2008_005928_fake_A_procd.png} &

\includegraphics[width=0.13\linewidth]{../Figures/2007_002273_real_B.png} &
\includegraphics[width=0.13\linewidth]{../Figures/2007_002273_real_A.png} &
\includegraphics[width=0.13\linewidth]{../Figures/2007_002273_fake_A_procd.png} \\

\end{tabular}
\caption{Results of employing \OurName for foreground extraction applied on horse photos from the HDSeg dataset. From left to right, we show the input image, the ground truth and \OurName's results.}
\end{figure*}
